# Supplementary material for: Question Generation from SQL Queries Improves Neural Semantic Parsing
Source: arXiv:1808.06304 source file (2018-08-27)
Supplement: Supplementary file 1 [file supplementary.pdf]

# Data Matters: Question Generation Improves Neural Semantic Parsing (Appendix)

Anonymous ACL submission


## Abstract

Due to the page limit of this paper submission, we describe some details in this appendix, including (1) the task of semantic parsing, (2) the STAMP model wed developed for question-to-SQL generation, and (3) the rule-based SQL sampler .


## A An Illustration of the Semantic Parsing Task

Figure 1 gives an example of semantic parsing. The task consists of two steps, which first maps a question to a SQL query and then executes the SQL query over the table to yield answer. Formally, the task takes a question $q$ and a table $t$ consisting of $n$ column names and $n \times m$ cells as the input, and outputs a SQL query $y$. We focus on question-to-SQL generation in this work.

## B An Illustration of the STAMP Model

Figure 2 illustrates an overview of the proposed STAMP model, which is short for Syntax- and Table- Aware seMantic Parser. As is shown, there are three "channels" in STAMP, among which the column channel predicts a column name, the value channel predicts a table cell and the SQL channel predicts a SQL keyword. At each time step, a switching gate selects a channel to predict a column name (maybe composed of multiple words), a cell (also maybe composed of multiple words) or a SQL keyword. The words in green above the SQL tokens stand for the results of the switching gate at each time step.

## C Rules of sampling SQL queries

To make the paper self-contained, we describe the SQL sampler we applied to both WikiSQL and WikiTableQuestions datasets. We use exactly the same SQL sampler shared by Zhong et al. (2017), which could be found at `https://github.com/salesforce/WikiSQL`. The SQL sampler adopts the following rules.

- The format of a SQL query is: *SELECT agg_op agg_col from table WHERE cond1_col cond1_op cond1 AND cond2_col cond2_op cond2 ...*
- The aggregation operator *agg_op* can be empty or *COUNT*. If the type of a aggregation column is numeric, the *agg_op* can additionally be one of *MAX* and *MIN*.
- The condition operator *cond_op* is $=$. If the type of a condition column is numerical, the *cond_op* can additionally be one of $>$ and $<$.
- The *cond* can be any cell value under the corresponding condition column *cond_col*. If the type of a condition column is numerical, *cond* can be numerical value sampled from the range the minimum value in the column to the maximum value in the column.
- The conditions will be removed if doing the action does not change the execution result.
- Besides, we only save the sampled SQL queries that produce non-empty result set.


## References

Victor Zhong, Caiming Xiong, and Richard Socher. 2017. Seq2sql: Generating structured queries from natural language using reinforcement learning. *arXiv preprint arXiv:1709.00103* .

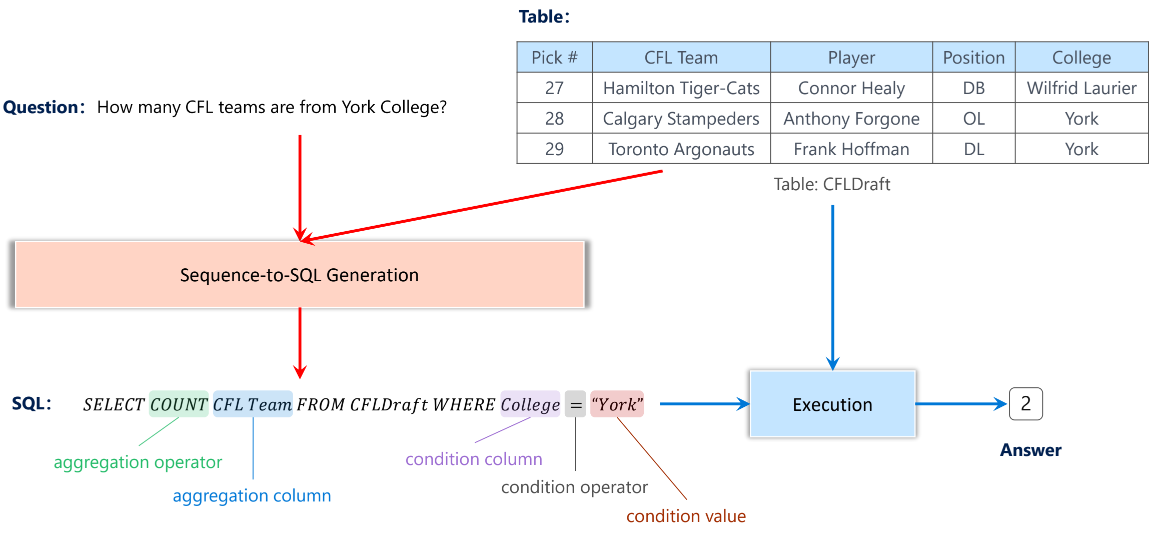


Figure 1: A brief illustrating of the semantic parsing task. The focus of this work is sequence-to-SQL generation

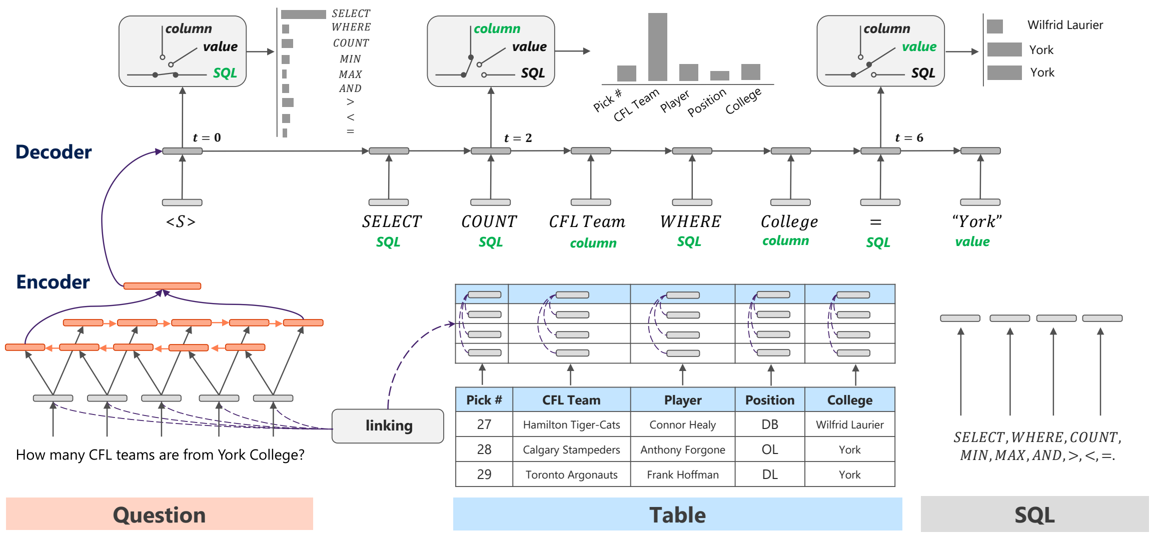


Figure 2: A brief illustrating of the proposed semantic parser (STAMP).
